# Supplementary material for: Metastability of Discrete-Symmetry Flocks
Source: arXiv:2306.01156 ancillary file (2023-06-01)
Supplement: Supplementary file 1 [file SM-v3.pdf]

# Supplemental Material for: "Metastability of Discrete-symmetry Flocks"

Brieuc Benvegnen,[1] Omer Granek,[2] Sunghan Ro,[3] Ran Yaacoby,[2] Hugues Chaté,[4,5,1] Yariv Kafri,[2] David Mukamel,[6] Alexandre Solon,[1] and Julien Tailleur[3]

[1] *Sorbonne Université, CNRS, Laboratoire de Physique Théorique de la Matière Condensée, 75005 Paris, France*
[2] *Department of Physics, Technion – Israel Institute of Technology, Haifa 32000, Israel*
[3] *Department of Physics, Massachusetts Institute of Technology, Cambridge, Massachusetts 02139, USA*
[4] *Service de Physique de l'Etat Condensé, CEA, CNRS Université Paris-Saclay, CEA-Saclay, 91191 Gif-sur-Yvette, France*
[5] *Computational Science Research Center, Beijing 100094, China*
[6] *Department of Physics of Complex Systems, Weizmann Institute of Science, Rehovot 7610001, Israel*

(Dated: June 1, 2023)

## CONTENTS

A. Numerical methods 1
1. Microscopic simulations of the AIM 1
a. Droplet dynamics 1
b. Measurement of the reversal probability 1
c. Late-time dynamics and sliding-window simulations 2
2. Numerical resolution of hydrodynamic equations 2
3. Supplementary figures 2
a. Threshold for droplet excitation 2
b. Spontaneous nucleation 3
4. Fig. 3b: Interface speeds 3
5. Fig. 3c: Droplet front 3

B. Newton mapping using the refined mean-field equations 4

References 4

## A. NUMERICAL METHODS

In this section, we detail our algorithms, protocols and post-processing schemes.

### 1. Microscopic simulations of the AIM

All our microscopic simulations were run using discrete-time Monte-Carlo algorithms with random-sequential updates.

#### a. *Droplet dynamics*

The simulations in which a droplet of oppositely moving particles is inserted in an ordered phase are run as follows. At time $t = 0$, we initialize the system by randomly distributing particles with spins $s = -1$ until a density $\rho_o$ is reached. After an equilibration time $t_r = 100$, a circular droplet of radius $r$—modulo lattice discretization effects—centered at $\mathbf{i} = (0, 0)$ is modified as follows. First, the spins located at sites within a distance $r$ from the center are set to $s = +1$. Second, an additional $\Delta N = (\rho_d^0 - \rho_o)\pi r^2$ particles with spins $s = +1$ are randomly distributed inside the droplet, leading to a droplet density $\rho_d^0 > \rho_o$ and a magnetization $\rho_d^0$. In Figs. 1(a-c), 2(b-c) and 3(c), we average the density and magnetization fields over 100 independent simulations.

#### b. *Measurement of the reversal probability*

We note that, when a droplet has grown significantly after having traveled a large enough distance, it almost surely takes over the entire ordered phase. To estimate $P_\mathrm{r}$, we thus proceeded as follows:

- We place a droplet with a positive magnetization in a negative-magnetization flock at $\mathbf{i} = (0, 0)$ as described in Section A 1 a.
- We record the magnetization of a $5 \times 5$ square region centered at $(\Delta x, 0)$ during a time interval $\Delta t = 4(\Delta x/v)$, with $\Delta x = 50$. This time is short enough to allow for good statistics, yet sufficiently long to assess whether the droplet has grown or receded after having traveled the distance $\Delta x$ from its seeding.
- If the average magnetization in the region increases by more than $\rho_o$ at any time during the measurement, we conclude that the droplet will keep growing and will eventually reverse the entire flock. $\Delta x$ is chosen to ensure the robust prediction of the droplet's fate.
- If the magnetization does not rise above the threshold by the end of the measurement at $t = t_r + 4(\Delta x/v)$, we conclude that the perturbation induced by the droplet will recede into the ordered phase.
- We repeat this protocol 100 times to estimate $P_\mathrm{r}$.

Note that we have checked that our results are not sensitive to the precise criteria used.

*c. Late-time dynamics and sliding-window simulations*

The longitudinal extent of the droplet and comet phases spread at a speed greater than $v(1+|p_o|)$. This makes the late-time regime very hard to reach numerically since one needs sizes such that $L_x > v(1+|p_o|)t$.

We thus developed an alternative scheme to produce the late-time data shown in Figs. 2(b) and 3(c) that allows us to use smaller system sizes. The method essentially consists in using a simulation box that travels with the droplet and we refer to it below as the 'Sliding-window method' (SWM). It consists in the following iterative steps:

1. We set an iteration counter $n = 0$ and initialize the droplet as in Sec. A 1 a in a system of size $(L_x(n), L_y(n)) = (3500, 200)$.

2. We run the simulation for a time $\Delta t$ such that the droplet travels a distance $L_x(0)/6$.

3. We measure the positions of the back ($x_+(n)$) and front ($x_{\rm f}(n)$) ends of the droplet, as well as its height $h(n)$. We then define a rectangular region $A(n)$ that contains all sites $(x, y)$ such that $x \in \{x_+(n) - 400, x_{\rm f}(n) + 100\}, y \in \{-h(n)/2 - 50, h(n)/2 + 50\}$. This region contains the whole droplet and its surrounding, but we chop the tail of the comet.

4. We prepare a new system of size $(L_x(n+1), L_y(n+1))$ in a homogeneous flocking phase, where
$$L_x(n+1) = L_x(0) + 500 + x_{\rm f}(n) - x_+(n)$$
$$L_y(n+1) = L_y(0) + 100 + h(n)\ .$$
To do so, we place randomly $\rho_o \cdot L_x(n+1) \cdot L_y(n+1)$ spins with $s = -1$ in the system and evolve them for a time $t_r = 100$. The exact configuration corresponding to the region $A(n)$ is then inserted in a region of identical size, centered at $(0, 0)$.

5. We set $n \to n+1$ and repeat from step 2, stopping when the desired time is reached.

We verified that the procedure yields droplets that are indistinguishable from those produced with the standard method described in Sec. A 1 a for times up to $t \simeq 2000$. (See the resulting magnetization fields and profiles in Fig. S1.) We then used the SWM to obtain data at longer times.

## 2. Numerical resolution of hydrodynamic equations

To solve the hydrodynamic Eqs. (1)-(2) of the main text, we use a pseudo-spectral integration scheme with

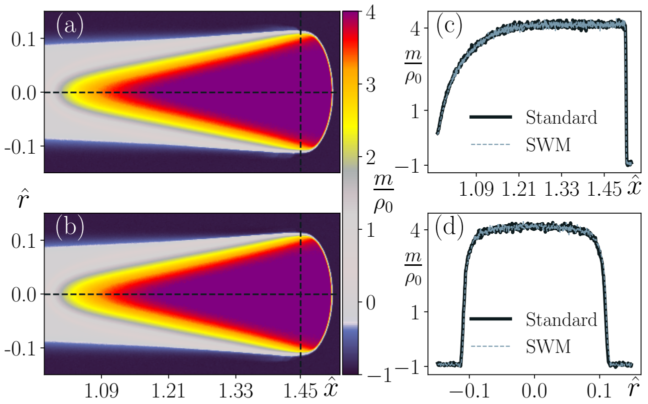


FIG. S1. **(a) - (b)** Droplets obtained using the standard procedure (a) and the SWM detailed in Sec. A 1 c (b), respectively. **(c) - (d)** Cross sections along $\hat{x}$ at $\hat{r} = 0$ (c) and along $\hat{r}$ at $\hat{x} = 1.45$ (d), measured using the standard procedure (black) and the SWM (cyan). Data were averaged over 100 realizations. Parameters: $t = 2020$, $D = v = 1$, and $\beta = 2$.

Euler time stepping and anti-aliasing with the standard 3/2 rule [1]. The initial condition is a counter-propagating circular droplet of radius $r$, introduced in an ordered phase of density $\rho_o = 1$ at $t = 0$. Its density is $\rho_d^0 = 12$ and its magnetization $m_d^0 > 0$ is the solution of the mean-field equation: $m_d^0/\rho_d^0 = \tanh \beta(m_d^0/\rho_d^0)$.

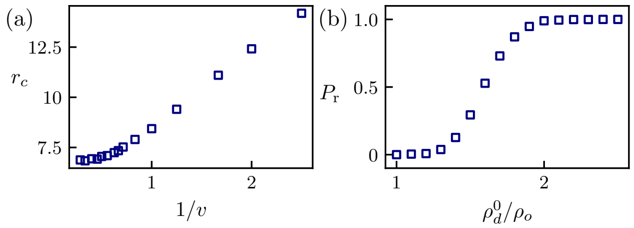


FIG. S2. **(a)** The nucleation critical radius, $r_c$, as a function of $1/v$. **(b)** The probability of reversing the ordered phase, $P_r$, for a droplet of initial radius 6 as a function of the droplet initial density $\rho_d^0$.

## 3. Supplementary figures

*a. Threshold for droplet excitation*

Figure S2(a) shows the threshold droplet size $r_c$ as a function of the inverse droplet speed $1/v$. Figure S2(b) shows $P_r$ as a function of $\rho_d^0$ for a fixed initial droplet radius $r = 6$.

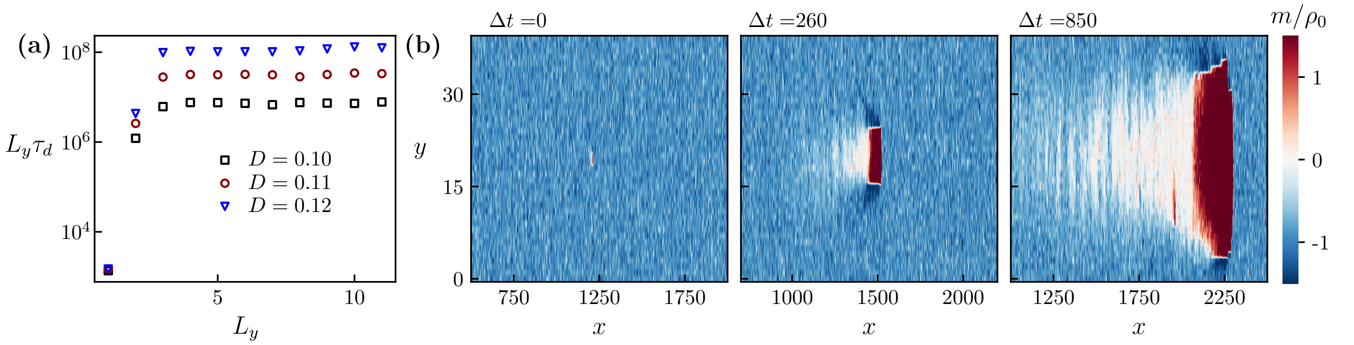


FIG. S3. **(a)** The average time required for a spontaneous nucleation to occur in the ordered phase of a system of size $200 \times L_y$ multiplied by $L_y$ as a function of $L_y$. **(b)** Snapshots of spontaneous nucleation showing a growing droplet. $\Delta t$ refers to the time elapsed since the initiation of the nucleation. Parameters: $\rho_o = 8$, $v = 1$ and $\beta = 2$ in all panels and $D = 0.1$ in panel (b).

*b. Spontaneous nucleation*

Figure 1(g) of the main text shows that the time taken for spontaneous droplet nucleation $\tau_d$ is inversely proportional to the area of the system. In Fig. S3(a), we present the dependence of the normalized nucleation time $L_y\tau_d$ measured in a narrow system of size $200 \times L_y$ while varying $L_y$ and $D$. As shown in the figure, the nucleation time first increases rapidly before saturating for large $L_y$. The saturated nucleation time increases exponentially with $D$. Finally, Fig. S3(b) shows snapshots of a spontaneous nucleation event.

### 4. Fig. 3b: Interface speeds

To compare the interface speeds measured in microscopic simulations with those predicted by the Newton mapping, we first simulated systems with $\beta = 2$, $L_x = 3000$, and $L_y = 300$. We prepared an initial condition corresponding to an ordered phase with a negative polarization, setting the average density to $\rho_o = 30$ and the spins to $s = -1$. Then, in a region of size $(7, L_y)$, we deposit particles at random until the density is $\rho_d^0 = 7\rho_o$ and set all the spins in the region to $s = +1$. This allows us to measure the speed of an interface with $\nabla_{\mathbf{r}_\perp} = 0$. The system is then evolved with the AIM Monte-Carlo simulations and we compare the positions of the band at $t = 70$ and $t = 230$. Interface positions are identified by locating points where the magnetization reaches the mean values between the phases connected by the interfaces. The interface speed is then calculated from the average speed between the two snapshots.

These numerically measured speeds are then compared with our theoretical predictions. The speeds of the $x_+$ and $x_-$ interfaces are given by their mean-field limits, $c_\pm = \pm v\rho_d$ (see Sec. B). To determine $c_\mathrm{f}$, we consider a left-going droplet and solve Eq. (5) of the main text, using $m = m_o$ and $m' = -10^{-6}$ as an initial condition. We then use dichotomy to find the value of $c$ that leads to a heterocline trajectory.

### 5. Fig. 3c: Droplet front

To compare the shape $\hat{x}(\hat{r})$ of the boundary layer separating the droplet and the ordered phase to the prediction of Eq. (11) of the main text, we first measure the density modulations inside the droplet using numerical simulations. To do this, we measure $\hat{r}$ cross-sections along the droplet, average them over 100 realizations, and fit the density modulations to a parabolic curve, as suggested by Eq. (11) (see Fig. S4). The curvatures $\kappa$ of these parabolic curves depend on $\hat{x}$ and is predicted to be of the form $\kappa(\hat{x}) = k/(\hat{x} - c_+)^2$. We then obtain an estimate for $k$ by fitting $\kappa(\hat{x})$ to this prediction using the value $c_+ = 0.95$ measured in the simulation (see Fig. S5).

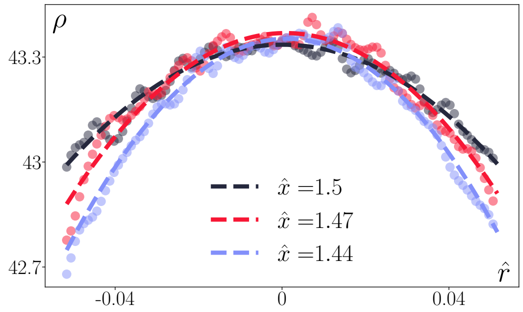


FIG. S4. Parabolic fits (dashed lines) of $\hat{r}$ cross-sections of the density field (circles) at different values of $\hat{x}$. The data was obtained using the SWM. Parameters: $D = v = 1$, $\rho_o = 10$, $\beta = 2$, $t = 4800$.

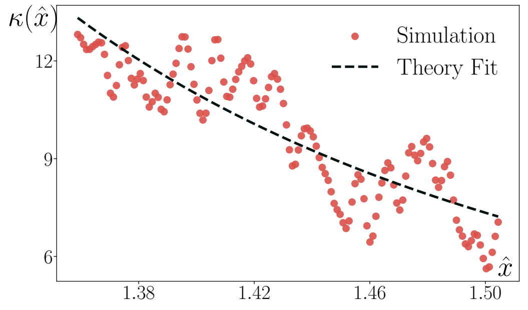


FIG. S5. Parabolic curvatures $\kappa(\hat{x})$ (red circles), as a function of $\hat{x}$, fitted to Eq. (10) of the main text (dashed black). The fit yields $k = 2.2 \pm 0.1$.

## B. NEWTON MAPPING USING THE REFINED MEAN-FIELD EQUATIONS

In this section we show that the Newton mapping allows identifying the fronts between the comet and its surrounding once we replace the mean-field expression of $F(\rho, m)$ by its refined-mean-field (RMF) counterpart:

$$F_{\rm RMF}(\rho, m) = F(\rho, m) - \alpha \frac{m}{\rho}\,, \tag{S1}$$

where $\alpha > 0$ is an unknown constant. We note that the model becomes ill-defined for $\beta > 3$ and higher-order corrections to mean-field are then needed [2]. To proceed, we use Eq. (5) of the main text, replacing $c_{\rm f}$ by $c = c_\pm$ and using $\partial_m V(m, c) = F_{\rm RMF}[\rho^0(m, c), m]$ for the effective force experienced by the fictitious particle. We note that $V(m)$ still has at most two maxima for $\beta < 3$.

Let us show that there are values of $c_\pm$ such that the Newton mapping admit heteroclinic solutions. For conciseness, we focus on the $x_+$ interface, which connects the disordered comet to the droplet. We remind that density, polarization, and magnetization in the droplet at $y = 0$ are denoted by $\rho_{\rm d}$, $p_{\rm d}$, and $m_{\rm d}$, respectively. We also note that fixed points of the Newton-mapping equations are dynamically stable solutions of the (refined) mean-field equations only if they are maxima of $V(m, c)$.

We now show that a heterocline exists for $c_+ \in [c^*_{\rm d}, c^*_{\rm c})$, with

$$c^*_{\rm d} = v p_{\rm d}\Big(1 - \frac{\alpha/2\rho_{\rm d}}{(\beta - 1 - \beta p_{\rm d} \tanh \beta p_{\rm d}) \cosh \beta p_{\rm d} - \alpha/2\rho_{\rm d}}\Big),$$

$$c^*_{\rm c} = v p_{\rm d}\Big(1 + \frac{\alpha/2\rho_{\rm d}}{\beta - 1 - \alpha/2\rho_{\rm d}}\Big)\,.$$

Let us consider a particle starting at $m = 0$ and $m' = 0^+$ for the two limiting cases $c = c^*_{\rm c,d}$ depicted in Fig. S6. For $c = c^*_{\rm c}$, a particle starting at $m = 0$ runs out to $m = -\infty$ because the $\partial^3_m V(m, c^*_{\rm c})|_{m=0} < 0$. For $c = c^*_{\rm d}$, $V(0) > V(m_{\rm d})$ so that a particle starting at $m = 0$ either runs out to $m = \infty$ or undergoes a supercritical relaxation to reach $m = m_{\rm d}$ at $t = +\infty$ (in which case $c_+ = c^*_{\rm d}$).

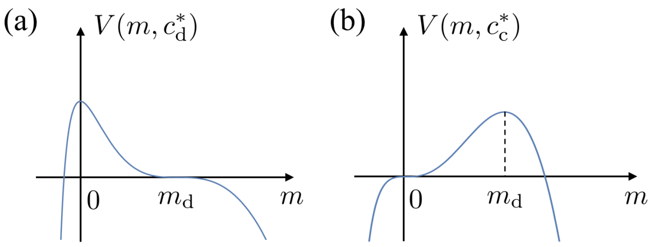


FIG. S6. Effective potential obtained from $F_{\rm RMF}$ at **(a)** $c_+ = c^*_{\rm d}$ and **(b)** $c_+ = c^*_{\rm c}$. Parameters: $v = 1$, $\beta = 2$, $\rho_{\rm d} = 4$, and $\alpha = 4$.

By continuity, there always exists a value of $c$ in $[c^*_{\rm d}, c^*_{\rm c})$ for which the friction provides or dissipates exactly the energy needed to reach $m = m_{\rm d}$. The precise value of $c_+$ can be found by dichotomy. In the mean-field limit used in the main text, $c^*_c$ and $c^*_d$ both converge to $v p_d$, which is the value used in Fig. 3(b) of the main text.

Following a similar procedure, the existence of the $x_-$ interface can also be demonstrated by finding the value of $c$ leading to a heterocline connecting the ordered phase $m = m_o$ to the disordered comet at $m = 0$. Finally, the front interface can also be analyzed using the RMF equations. This leads to a correction to the mean-field prediction of order $\alpha/\rho_o$, which is negligible in the large $\rho_o$ regime explored in our letter.


[1] B. Fornberg, *A practical guide to pseudospectral methods*, 1 (Cambridge university press, 1998).

[2] A. P. Solon and J. Tailleur, Physical Review E **92**, 042119 (2015).
